# Supplementary material for: Black-Box Uncertainty Estimation for Deep Learning Models in Atomistic Simulations
Source: arXiv:2511.16439 ancillary file (2025-11-20)
Supplement: Supplementary file 1 [file manuscript_SI.pdf]

# Supporting Information for: Black-Box Uncertainty Estimation for Deep Learning Models in Atomistic Simulations

Idan Fonea,[*,†] Amir Peles,[†] Sivan Niv,[†] Goren Gordon,[‡,¶] and Amir Natan[*,†,§]

†*Department of Physical Electronics, School of ECE, Tel Aviv University, Israel*

‡*School of Industrial Engineering and Intelligent Systems, Tel Aviv University, Israel*

¶*Luddy School of Informatics, Computing, and Engineering, Indiana University Bloomington, Bloomington, IN, USA*

§*The Sackler Center for Computational Molecular and Materials Science, Tel Aviv University, Israel*

E-mail: idanfonea@gmail.com; amirnatan@post.tau.ac.il

## S1 Deep Learning Model Details

In this section, we show the details of the deep learning model which is used for the analysis in the main text. The model is a direct force model, which is an improvement of the model developed by Kuritz et al.[1] that uses embedding to ensure permutation invariance and data augmentation to ensure rotation invariance. We adapt the approach used by Zhang et al.[2] to process the input in the following way: first we define a cutoff radius around each atom and find the $k$ nearest neighbors inside this radius. We then define the following smoothing function:

$$s(r_{ji}) = \begin{cases} \frac{1}{r_{ji}}, & r_{ji} < r_{cs}, \\ \frac{1}{r_{ji}} \left\{ \frac{1}{2} \cos\left[ \pi \frac{(r_{ji} - r_{cs})}{(r_c - r_{cs})} \right] + \frac{1}{2} \right\} & r_{cs} < r_{ji} < r_c, \\ 0, & r_{ji} > r_c. \end{cases} \tag{S1}$$

The neighbors information is then mapped to $\widetilde{R}^i$, such that for each neighbor $j$ we have:

$$\widetilde{R}^i_j = \{s(r_{ji}), \hat{x}_{ji}, \hat{y}_{ji}, \hat{z}_{ji}\} = \left\{ s(r_{ji}), \frac{s(r_{ji})x_{ji}}{r_{ji}}, \frac{s(r_{ji})y_{ji}}{r_{ji}}, \frac{s(r_{ji})z_{ji}}{r_{ji}} \right\} \tag{S2}$$

The data in Eq.S2 is then transformed into a new features vector, $D^i$, by:

$$D^i = (\mathcal{G}^i)^T \widetilde{R}^i \tag{S3}$$

Similarly to Zhang et al.[2], the matrix $\mathcal{G}(s(r_{ji}))$ is created by a helper network (called the embedding network) that gets as an input the single value of $s(r_{ji})$ and produces $M$ outputs. The embedding matrix is generated through a machine learning process and learns an optimal set of radial basis functions for the given database. The original dimension of $\widetilde{R}^i$ is $K \times 4$, where $K$ is the number of neighbors. The dimension of $D^i$ is $M \times 4$. The new features, $D^i$, are then fed into a dense neural network that produces the prediction of the force vector $\vec{F}$ for the atom $i$. Eq. S3 ensures invariance of the model under atom permutation. The model is trained with the data being randomly rotated, hence creating rotation indifference of the model via data augmentation. The model parameters for sodium are: $K = 100$, $r_{cs} = 5.8, r_c = 6.0$, the embedding network is $80 \times 40$, the dense network is $500 \times 250$. The model parameters for aluminum are: $K = 100$, $r_{cs} = 5.5, r_c = 6.0$, the embedding network is $80 \times 40$, the dense network is $500 \times 250$.

## S2 Results for a wider range of temperatures

Here, we show the results of the Na300 K and Na2000 K trained models for additional test temperatures ranging from 100 K to 4000 K. In Figures S1 and S2 (sodium and aluminum respectively) we observe that the $UQ_d$ signal is correlated with the magnitude of the force, displaying a monotonic relationship with the test temperatures, this trend is similar to what is shown in the manuscript for only 300 K and 2000 K. In figures S3 and S4 (sodium and aluminum respectively) we show the increase in the likelihood of OOD detection with the distance of the test dataset from the training dataset, again in a similar fashion to what is shown in the main text for only two temperatures. In figures S5 and S6, we show for sodium and aluminum bulk, respectively, the behavior of $UQ_d$ and $UQ_r$ against $AE$ and $AE_r$ on a logarithmic scale for visual comparability, to capture the relations of all the signals to each other

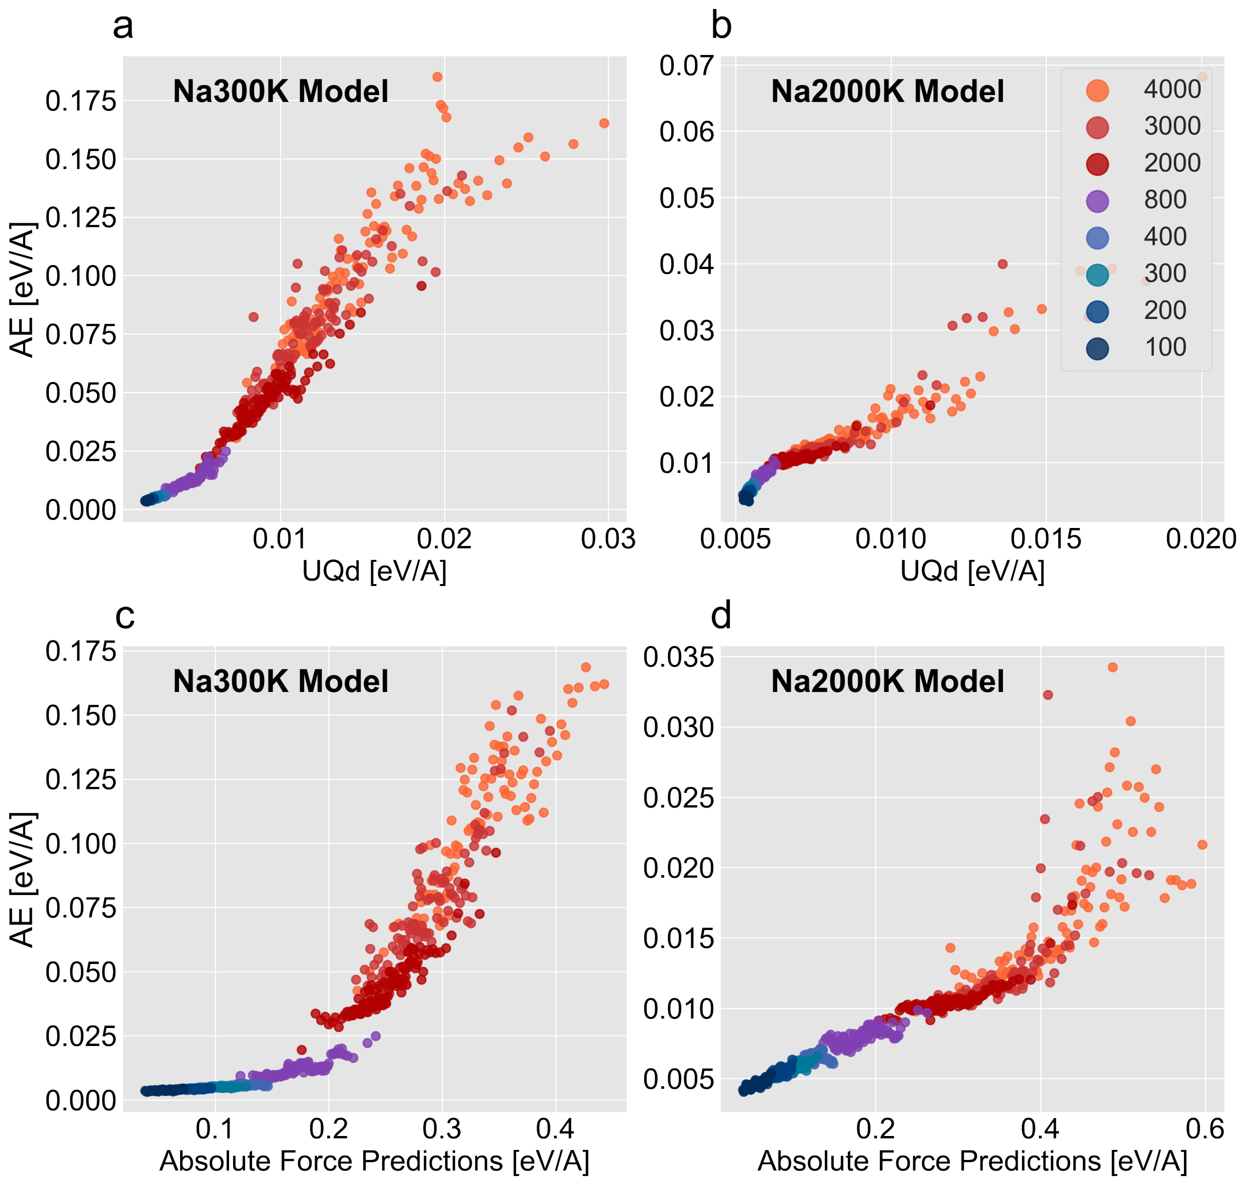


Figure S1: Panels (a, b) show a scatter plot of the AE (Eq.2) against the $UQ_d$ signal (Eq.4) produced for the Na300 K (a) and the Na2000 K (b) trained models, tested on datasets from 100 K to 4000 K. Panels (c,d) show a scatter plot of the AE (Eq.2) against the average absolute predicted force (Eq.9) for models trained on Na300 K (c) and Na2000 K (d). In all sub figures, the data is sorted according to the x-axis, then grouped into 100 bins where the AE is averaged in each bin.

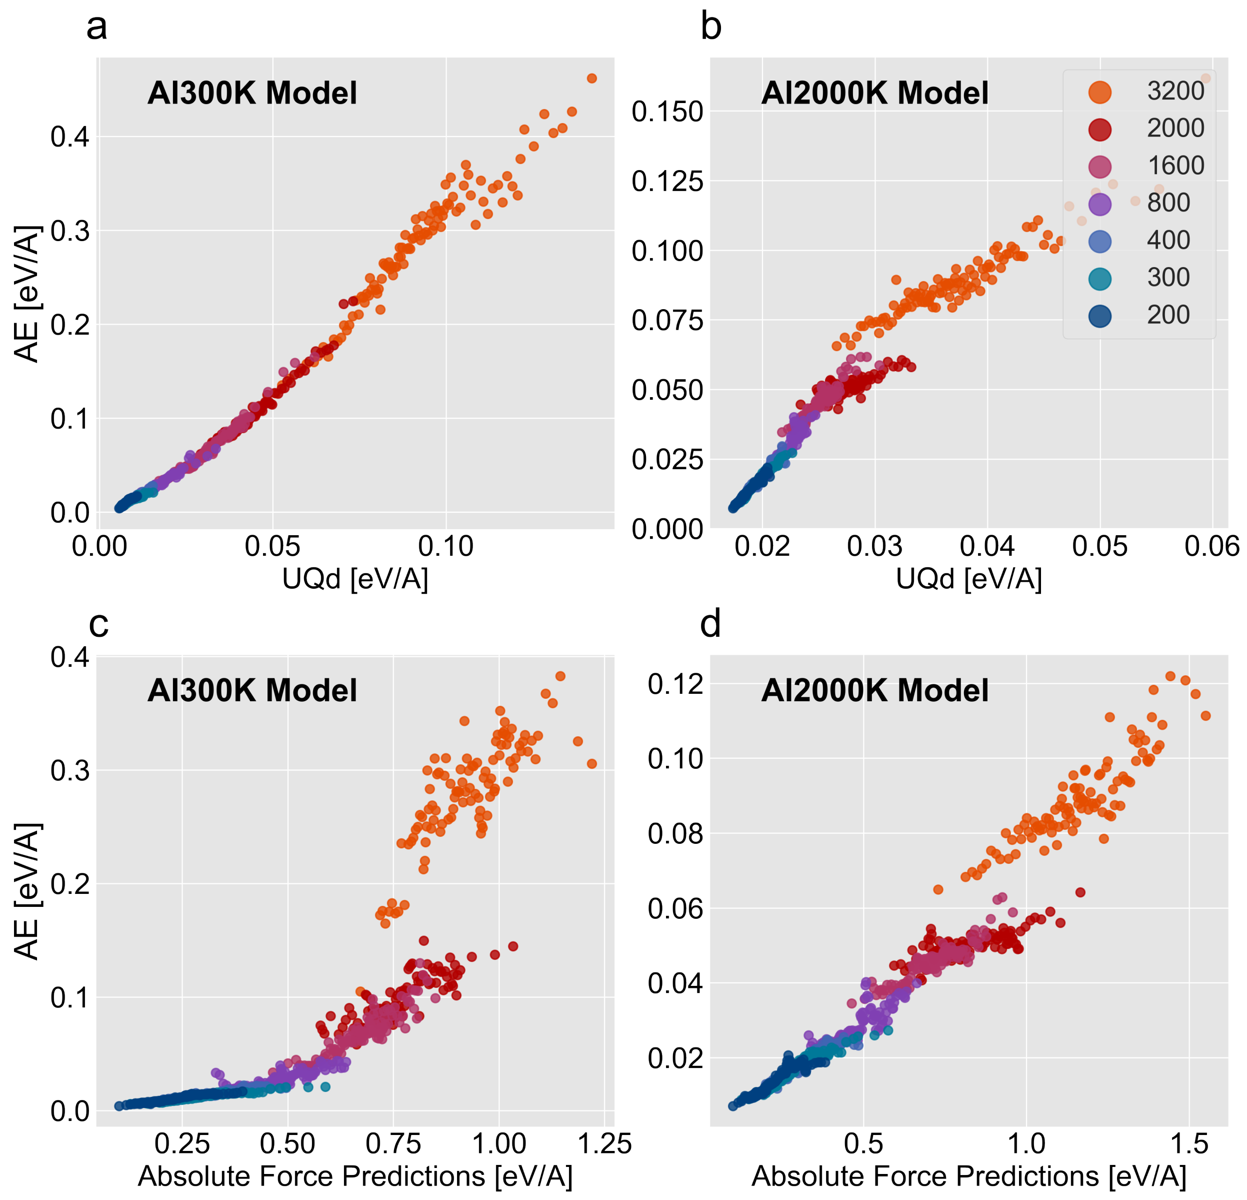


Figure S2: Panels (a, b) scatter plot of the AE (Eq.2) against the $UQ_d$ signal (Eq.4) produced for the Al300 K (a) and the Al2000 K (b) trained models, tested on data from 100 K to 3200 K. Panels (c,d) show a scatter plot of the AE (Eq.2) against the average absolute predicted force (Eq.9) for models trained on Al300 K (c) and Al2000 K (d). In all sub figures, the data is sorted according to the x-axis, then grouped into 100 bins where the AE is averaged in each bin.

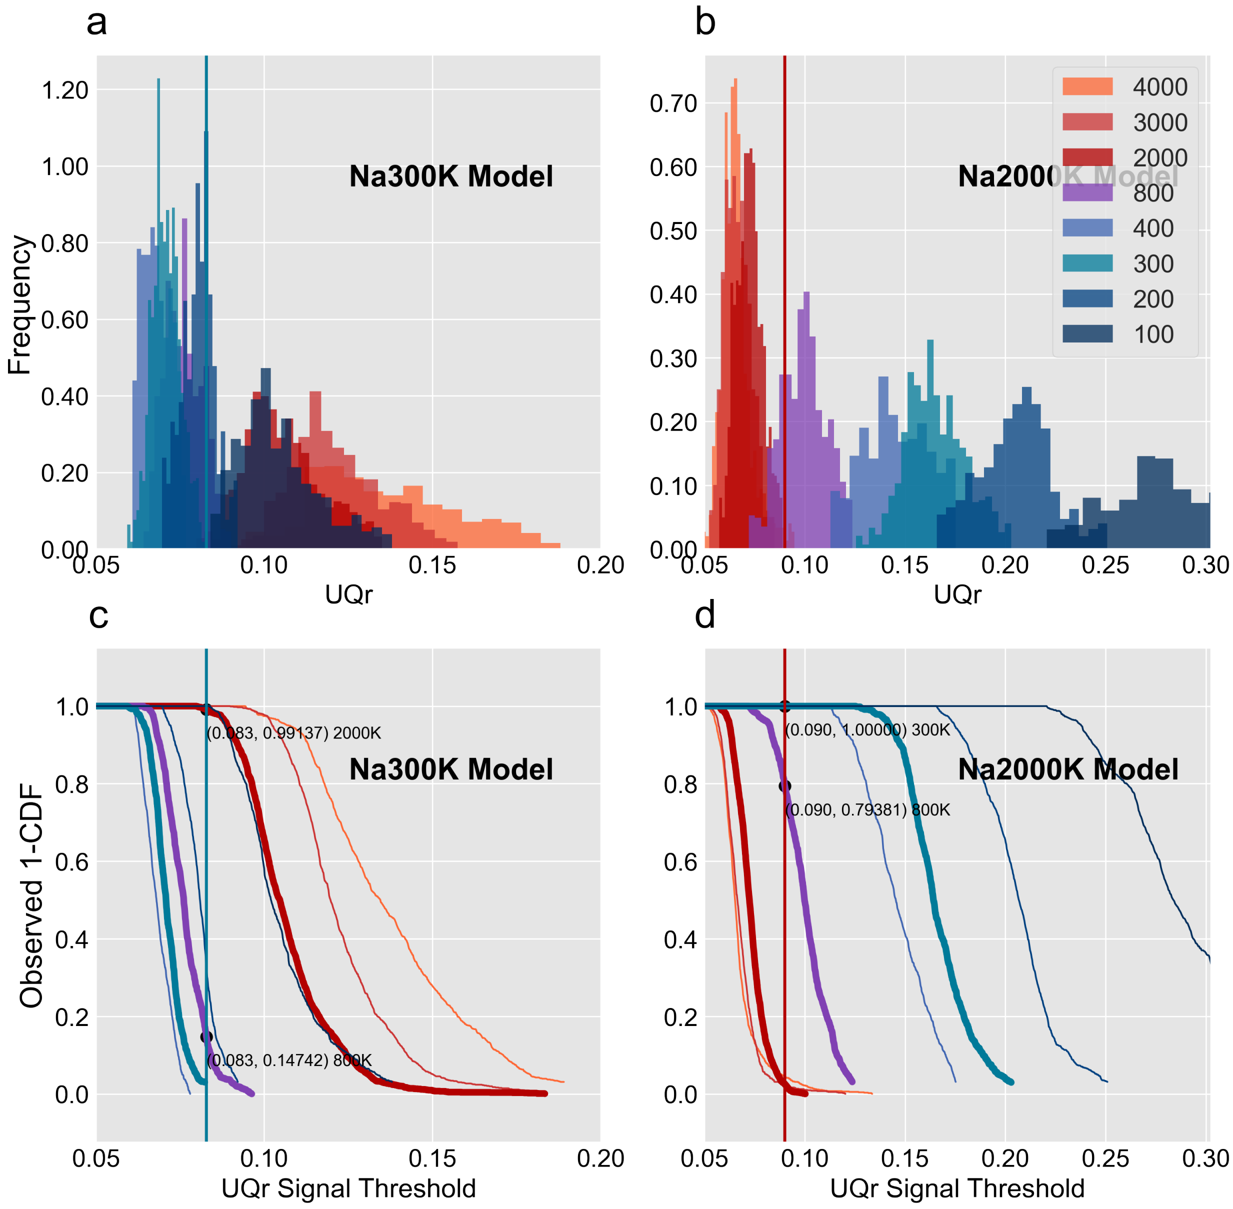


Figure S3: In (a, b) - Distribution of the $UQ_r$ (Eq.9) for Na300 K (a) and the Na2000 K (b) trained models, tested on temperatures from 100 K to 4000 K data, in bins of 0.01. In (c,d) - The observed cumulative density function (CDF) obtained from Eq.13 measuring the frequency of $UQ_r$ signal samples that are above a threshold set at that point. The results for Na300 K, Na800 K and Na2000 K are in bold. The vertical line is set on the $97.5^{th}$ percentile of the relative uncertainty (which is equivalent to $P_{\text{OOD}} = 0.025$) on the train temperature of Na300 K (a,c) and Na2000 K (b,d).

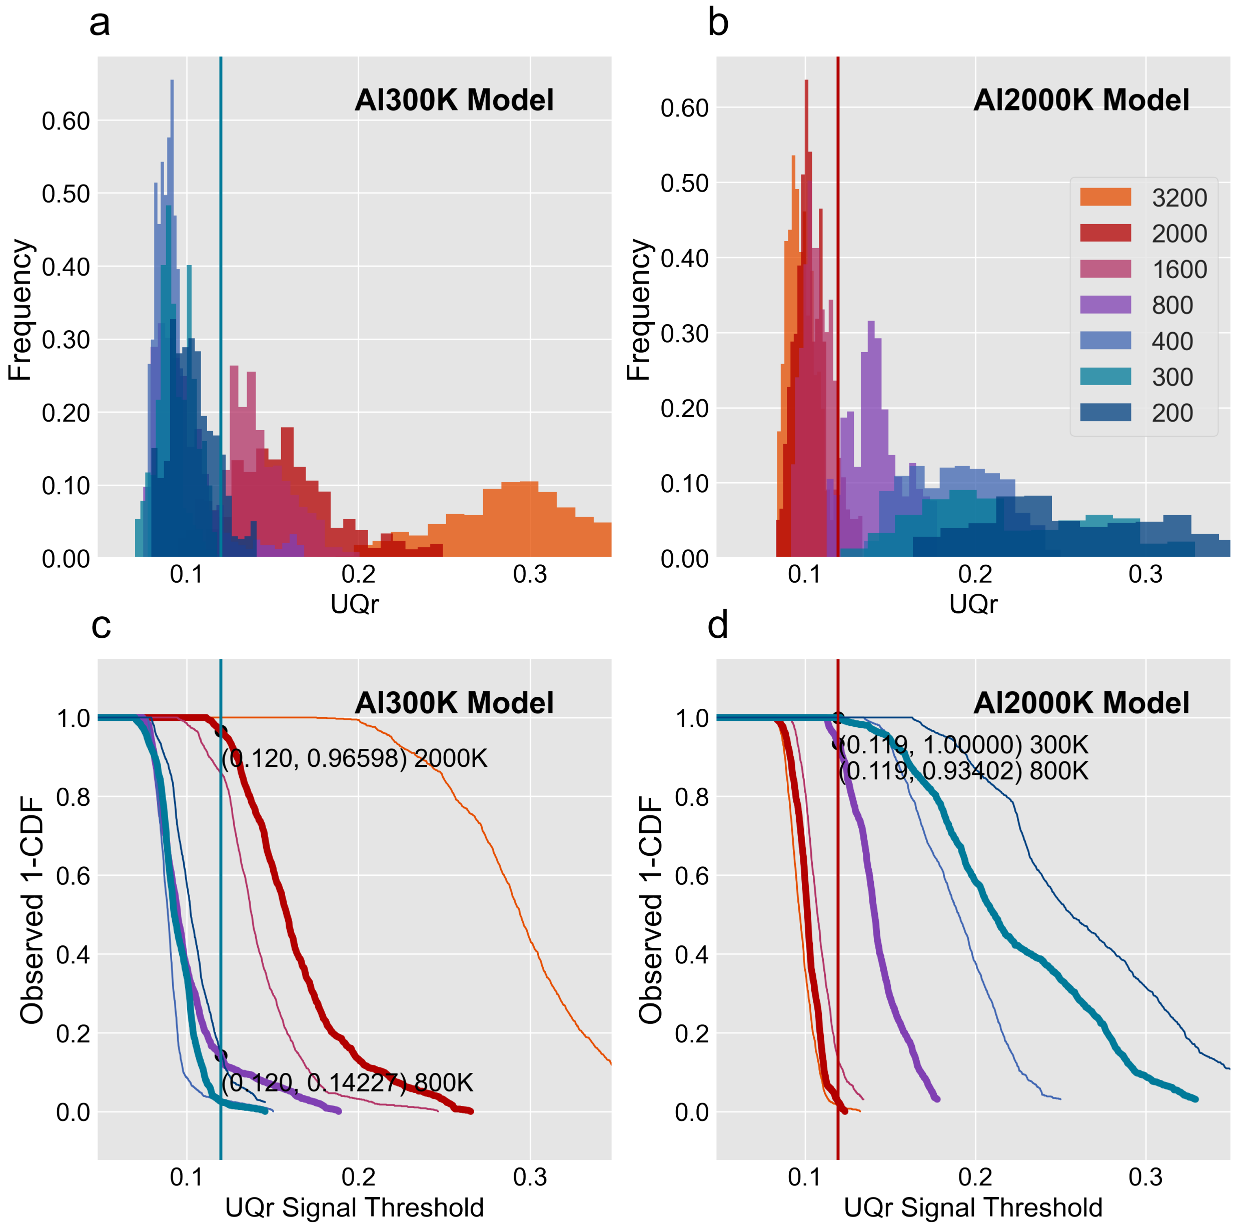


Figure S4: In (a, b) - Distribution of the $UQ_r$ (Eq.9) for Al300 K (a) and the Al2000 K (b) trained models, tested on 200 K to 3200 K data, in bins of 0.01. In (c,d) - The observed cumulative density function (CDF) obtained from Eq.13 measuring the frequency of $UQ_r$ signal samples that are above a threshold set at that point. The results for 300 K, 800 K and 2000 K are shown in bold. The vertical line is set on the $97.5^{th}$ percentile of the relative uncertainty on (which is equivalent to $P_{\text{OOD}} = 0.025$) on the train temperature of Al300 K (a,c) and Al2000 K (b,d).

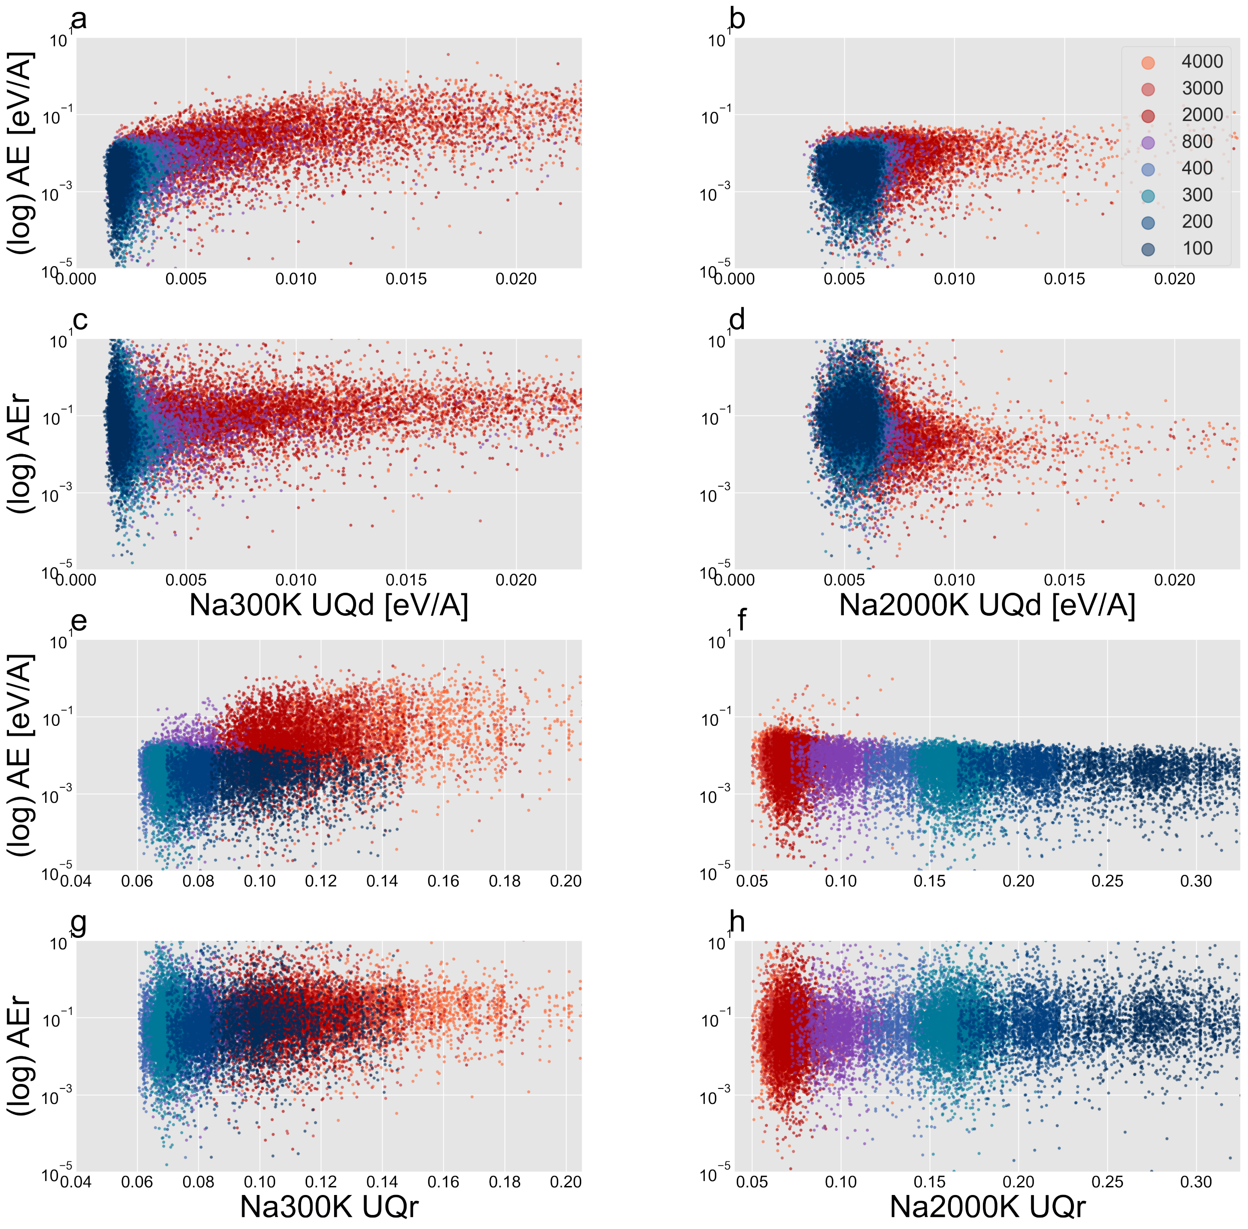


Figure S5: The $UQ_d$ and the $UQ_r$ behavior of models trained on Na300 K (a,c,e,g) and Na2000 K (b,d,f,h) and tested on 8 different temperature datasets, from 100 K to 4000 K. To improve visual separation, the $UQ_r$ signal was normalized as in Eq.9 using $W_n$ of 5, and both the $UQ_r$ and the $UQ_d$ signals were smoothed as in Eq.10 using $W_u$ of 5. The top sub-figures pair (a,b) show the $UQ_d$ signal (Eq.4), against the Absolute Error (AE Eq.2) on a logarithmic scale. In the second sub figures pair (c,d), we show the $UQ_d$ signal against the Relative AE, ($AE_r$) (Eq.5).In the following sub figures pair (e,f), we show the $UQ_r$ signal against the AE (Eq.2). In the bottom sub figures pair (c,d), we show the $UQ_r$ against the Relative AE, $AE_r$ (Eq.5).

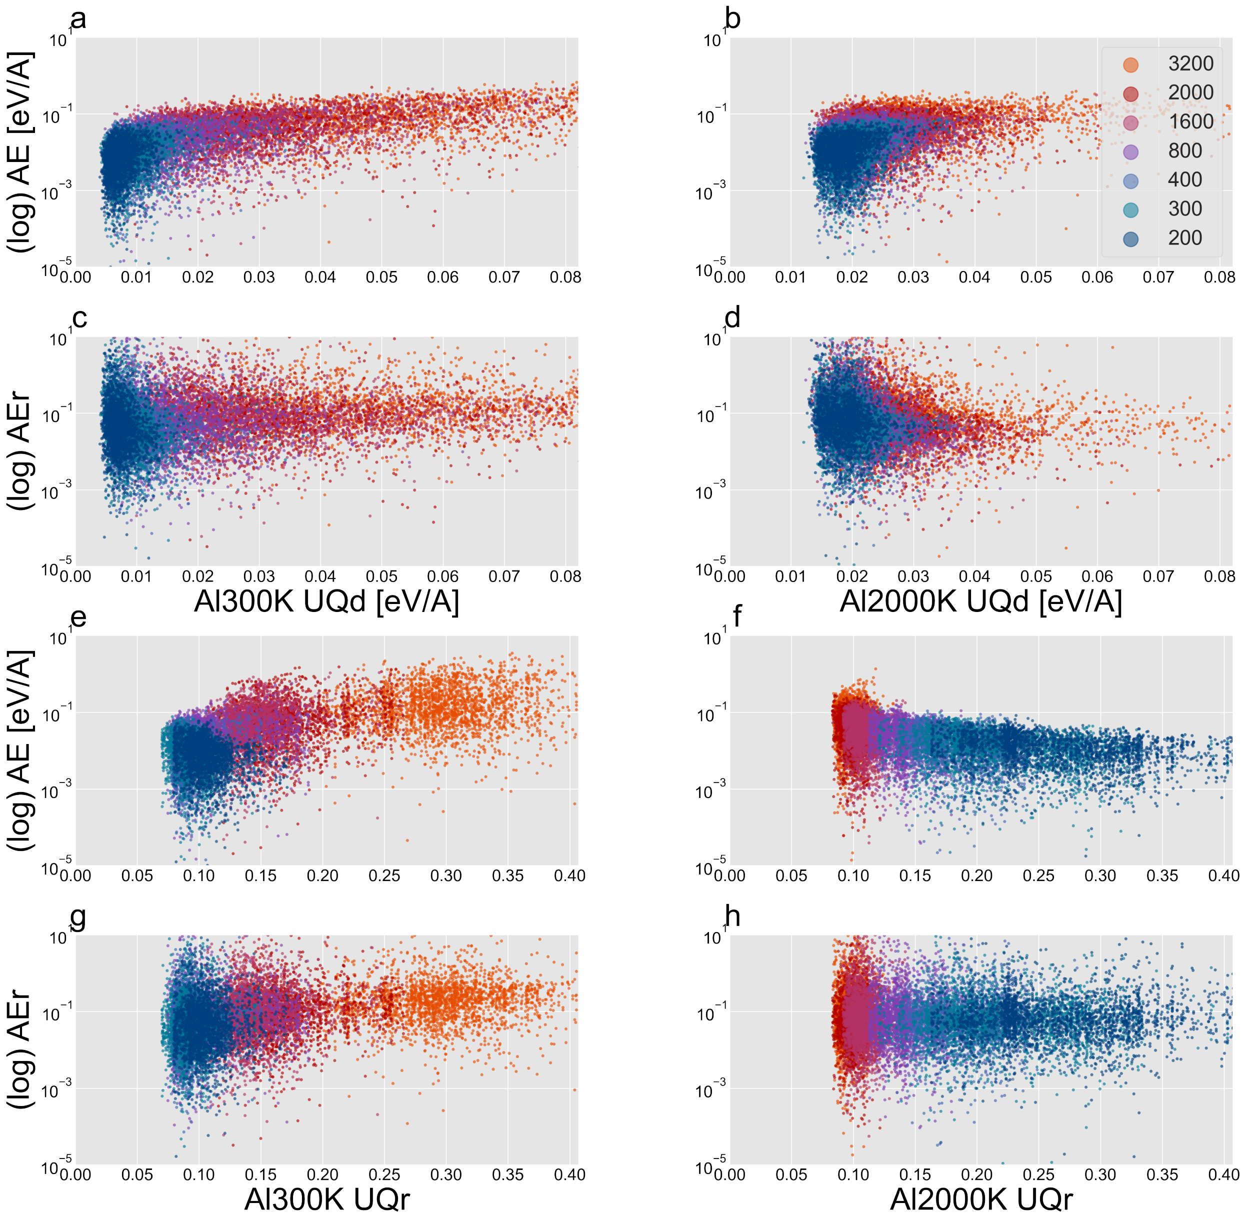


Figure S6: The $UQ_d$ and the $UQ_r$ behavior of models trained on Al300 K (a,c,e,g) and Al2000 K (b,d,f,h) and tested on 7 different temperature datasets, from 200 K to 3200 K . Smoothing and normalization was done similarly to the Sodium case. The $UQ_r$ signal was normalized as in Eq.9 using $W_n$ of 5, and both the $UQ_r$ and the $UQ_d$ signals were smoothed as in Eq.10 using $W_u$ of 5. The top sub-figures pair (a,b) show the $UQ_d$ signal (Eq.4), against the Absolute Error (AE Eq.2) on a logarithmic scale. In the second sub figures pair (c,d), we show the $UQ_d$ signal against the Relative AE, ($AE_r$) (Eq.5).In the following sub figures pair (e,f), we show the $UQ_r$ signal against the AE (Eq.2). In the bottom sub figures pair (c,d), we show the $UQ_r$ against $AE_r$ (Eq.5).

Table S1 summarizes the performance of the models across the extended temperature

Table S1: Extended cross-temperature performance metrics for Na and Al materials. The table reports prediction error (MAE, $MAE_r$) and uncertainty metrics ($UQ_d$, $UQ_r$), $P_{\text{OOD}}$, together with the true and predicted force average norms $\|\vec{F}^{DFT}\|$ and $\|\vec{F}^{Pred}\|$.

| X | Train($K$) | Test($K$) | MAE | $MAE_r$ | $UQ_d$ | $UQ_r$ | $P_{\text{OOD}}$ | $\|\vec{F}^{DFT}\|$ | $\|\vec{F}^{Pred}\|$ |
|---|---|---|---|---|---|---|---|---|---|
| Na | 300 | 100 | 0.0038 | 0.4093 | 0.0019 | 0.1052 | 1.000 | 0.055 | 0.055 |
| | | 200 | 0.0042 | 0.3145 | 0.0020 | 0.0808 | 0.328 | 0.080 | 0.080 |
| | | 300 | 0.0048 | 0.2788 | 0.0023 | 0.0713 | 0.025 | 0.099 | 0.099 |
| | | 400 | 0.0054 | 0.3210 | 0.0025 | 0.0683 | 0.000 | 0.114 | 0.114 |
| | | 800 | 0.0121 | 0.3494 | 0.0043 | 0.0764 | 0.147 | 0.179 | 0.173 |
| | | 2000 | 0.0444 | 0.4149 | 0.0088 | 0.1067 | 0.991 | 0.288 | 0.251 |
| | | 3000 | 0.0766 | 0.5740 | 0.0117 | 0.1227 | 1.000 | 0.358 | 0.289 |
| | | 4000 | 0.1053 | 0.6171 | 0.0151 | 0.1381 | 1.000 | 0.423 | 0.328 |
| | 2000 | 4000 | 0.0162 | 0.2244 | 0.0092 | 0.0673 | 0.043 | 0.423 | 0.417 |
| | | 3000 | 0.0128 | 0.2809 | 0.0077 | 0.0676 | 0.022 | 0.358 | 0.355 |
| | | 2000 | 0.0104 | 0.2476 | 0.0067 | 0.0730 | 0.025 | 0.288 | 0.287 |
| | | 800 | 0.0079 | 0.3102 | 0.0058 | 0.1004 | 0.794 | 0.179 | 0.180 |
| | | 400 | 0.0062 | 0.3692 | 0.0055 | 0.1462 | 1.000 | 0.114 | 0.116 |
| | | 300 | 0.0058 | 0.3227 | 0.0054 | 0.1666 | 1.000 | 0.099 | 0.100 |
| | | 200 | 0.0054 | 0.3823 | 0.0054 | 0.2067 | 1.000 | 0.080 | 0.082 |
| | | 100 | 0.0046 | 0.4940 | 0.0053 | 0.2939 | 1.000 | 0.055 | 0.056 |
| Al | 300 | 200 | 0.0105 | 0.2817 | 0.0076 | 0.1050 | 0.147 | 0.230 | 0.230 |
| | | 300 | 0.0117 | 0.2870 | 0.0088 | 0.0949 | 0.026 | 0.289 | 0.289 |
| | | 400 | 0.0153 | 0.2648 | 0.0099 | 0.0904 | 0.030 | 0.334 | 0.334 |
| | | 800 | 0.0279 | 0.3620 | 0.0160 | 0.1012 | 0.142 | 0.484 | 0.480 |
| | | 1600 | 0.0692 | 0.5460 | 0.0320 | 0.1418 | 0.860 | 0.714 | 0.676 |
| | | 2000 | 0.0971 | 0.4193 | 0.0413 | 0.1642 | 0.966 | 0.824 | 0.761 |
| | | 3200 | 0.2779 | 0.8287 | 0.0902 | 0.2946 | 1.000 | 1.147 | 0.921 |
| | 2000 | 3200 | 0.0887 | 0.5848 | 0.0372 | 0.0979 | 0.015 | 1.147 | 1.156 |
| | | 2000 | 0.0499 | 0.3648 | 0.0271 | 0.1017 | 0.026 | 0.824 | 0.821 |
| | | 1600 | 0.0452 | 0.5093 | 0.0251 | 0.1090 | 0.134 | 0.714 | 0.709 |
| | | 800 | 0.0282 | 0.3722 | 0.0219 | 0.1431 | 0.934 | 0.484 | 0.476 |
| | | 400 | 0.0188 | 0.3001 | 0.0199 | 0.1907 | 1.000 | 0.334 | 0.326 |
| | | 300 | 0.0161 | 0.3359 | 0.0194 | 0.2240 | 1.000 | 0.289 | 0.282 |
| | | 200 | 0.0136 | 0.3593 | 0.0188 | 0.2706 | 1.000 | 0.230 | 0.225 |

range (100 K to 4000 K). As expected, models trained at low temperatures (300 K) exhibit a significant increase in MAE when tested at higher temperatures. This degradation in performance is accompanied by a systematic underestimation of the force norms ($\|\vec{F}^{\mathrm{Pred}}\|$ vs $\|\vec{F}^{\mathrm{DFT}}\|$), particularly in the highest temperature regimes (e.g., Na at 4000 K and Al at 3200 K). Conversely, models trained at 2000 K demonstrate robust performance, maintaining relatively low MAE values and accurate force norm predictions across the entire temperature spectrum. We observe asymmetry in the model performance and response of $UQ_r$ in the direction of distancing up and down from the train temperature. Crucially, the proposed uncertainty metrics effectively capture these trends. As seen in Figures S5 and S6, the direct uncertainty signal ($UQ_d$) correlates strongly with the absolute error (AE) across multiple orders of magnitude for both Na and Al. Furthermore, the $UQ_r$ successfully identifies the different temperature regimes as out-of-distribution (OOD) for the Na 300 K model and same for the Na 2000 K model.

# S3 Additional slab results

Here we show more results of a model trained on an aluminum bulk of 300 K tested on a slab configuration of 300 K as well. In Figure 7 of the manuscript, we show the directional, per atom, MAE and $UQ_r$ as a function of atom index for all 3 directions. Here we also show the $MAE_r$ and MAPE values in Figures S7 and S8 respectively. We show the MAPE to exhibit the extremely high magnitude of the predicted force in relation to the true value. The MAPE value is calculated according to Eq. S4.

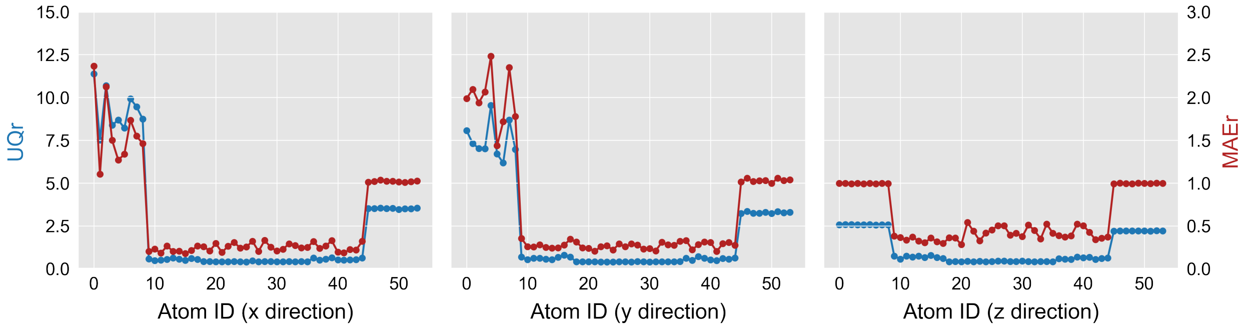


Figure S7: Relative uncertainty (UQ) of an aluminum model trained on 300K bulk configuration, and tested on 300K slab configuration (right axis, in red) and corresponding $MAE_r$ (left axis, in blue). The $UQ_r$ is calculated using Eq.9 without smoothing over the directions and over the atom in the cell, else smoothed only over samples in time, to isolate the directional atomwise components

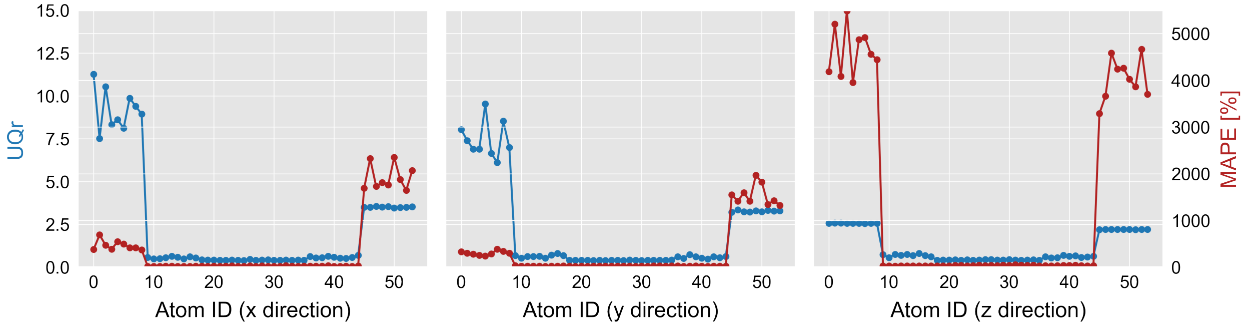


Figure S8: Showing also the MAPE to exhibit the extremely high magnitude of the predicted force in relation to the true value. Results of a model trained on 300 K bulk configuration, and tested on 300 K slab configuration. The $UQ_r$ is on the left axis in blue and the corresponding MAPE is on the right axis in red. The $UQ_r$ and the normalization is calculated using Eq.9 .

We define the mean absolute percentage error (MAPE), in a similar way as the $MAE_r$ for a special case of averaging over the consecutive samples (not over the direction and other atoms in the cell). We calculate the absolute percentage error (APE) using the true labels ($\vec{F}_{i,a}^{DFT}$) as the denominator instead of the predictions. Here, $\delta$ is also chosen as $10^{-2}eV/\mathring{A}$. We then derive the MAPE by averaging the APE on the samples of the test set of size $S$ as in Eq. S4 .

$$MAPE_{a,\beta} = \frac{1}{S}\sum_{i=1}^{S}\frac{|\overline{F}_{i,a} - F_{i,a}^{DFT}|}{|F_{i,a}^{DFT}| + \delta} \tag{S4}$$

where $i$ is the sample index , $a$ is the atom index and $\beta$ is the Cartesian direction.

## References


(1) Kuritz, N.; Gordon, G.; Natan, A. Size and temperature transferability of direct and local deep neural networks for atomic forces. *Phys. Rev. B* **2018**, *98*, 094109.

(2) Zhang, L.; Han, J.; Wang, H.; Saidi, W.; Car, R.; E, W. End-to-end symmetry preserving inter-atomic potential energy model for finite and extended systems. *Adv. Neural Inf. Process. Syst.* **2018**, *31*.
